# Supplementary material for: Container: Context Aggregation Network
Source: arXiv:2106.01401 source file (2021-10-18)
Supplement: Supplementary file 1 [file 99_appendix.tex]

\section*{Appendix}

\setcounter{table}{0}

\setcounter{figure}{0}

\setcounter{algocf}{0}

\section{Experimental setups}

\subsection{ImageNet Classification}
ImageNet-1k is an image classification dataset with 1000 object categories. We use the basic architecture explained in Section~\ref{approach:container_net}. 
% and replace the contextual aggregation module with Depthwise convolution, transformer, MLP, \model, and \modellight module. For PAM, we place PAM module directly into the self-attention module in DeiT. Our model has near 20M parameters to have a fair comparison with DeiT-small and ResNet-50 models. 
All models are trained with the same setting as DeiT. Depthwise convolution, MLP and \modellight are trained with 8 16G V100 GPU with each GPU processing 128 images. Transformer and \model are trained with 8 80G A100 GPU and each GPU processes 128 images. Color jitter, random erase and mixup are used as data-augmentation strategies. We use the adamW optimizer. Learning rates are calculated using the following equation:
\begin{align}
    lr = \frac{lr_{base} \times Batch \times N_{GPU}}{512}
\end{align}   
where base learning rate is chosen to be $5 \times e^{-4}$. We use cosine learning schedule and warm up the model in the first 5 epochs and train for 300 epochs in total. 

\subsection{Detection with RetinaNet}
RetinaNet is a one-stage dense object detector using a feature pyramid network and focal loss. It is trained for 12 epochs, starting with a learning rate of 0.0001 which decreases by 10 at epoch 8 and 11. We use adamW optimizer and set weight decay to 0.05. No gradient clip is applied. We warm up for the first 500 iterations. Models are trained with 8 V100 GPU and each GPU holds 2 images. We freeze the batch normalization parameter similar to DETR.

\subsection{Detection and Segmentation with Mask-RCNN}
Mask-RCNN is a multi-task framework for object detection and instance segmentation. Mask-RCNN models are trained with 8 GPUs and each GPU hold 2 images. Mask-RCNN models are optimized by AdamW with a learning rate of 0.0001 and weight deacy of 0.05. We warm up the first 500 iterations. BN parameters are frozen for all layers. 

\subsection{Detection with DETR}
DETR is an encoder-decoder transformer for end-to-end object detection. To improve the convergence speed and performance of DETR, SMCA-DETR propose a spatial modulated co-attention mechanism which can increase the convergence speed of DETR. Deformable DETR achieve fast convergence through deformable encoder and decoder. We compare \modellight with ResNet 50 on DETR without dilation, SMCA without multi scale and Deformable DETR without multi scale. DETR and SMCA DETR are optimized with 8 GPUs and 2 images per GPU, where as Deformable DETR uses 8 GPUs and 4 images per GPU. All models are optimzied with AdamW optimizer and weight clipping. DETR, SMCA DETR and Deformable DETR all use the default parameter setting in the original code release. 

\begin{table}[h!]
\setlength\tabcolsep{2pt}
    \centering
    \begin{tabular}{c|ccccccccc}
        \toprule
        Method & Backbone  & mAP & AP$_S$ & AP$_M$ & AP$_L$\\
        \midrule
        DETR~\cite{carion2020end} &ResNet50  & 32.3 &10.7& 33.8&53.0 &\\
        DETR~\cite{carion2020end} &\modellight  & 38.9 &16.5&  42.2&60.3 &\\
        \midrule
        \makecell[c]{SMCA w/o\\ multi-scale~\cite{gao2021fast}} & ResNet50 &  41.0 &21.9& 44.3&59.1\\
        \makecell[c]{SMCA w/o\\ multi-scale~\cite{gao2021fast}} & \modellight &  44.2 & 23.8& 47.9&63.1\\
        \midrule
        \makecell[c]{DDetr w/o\\ multi-scale~\cite{zhu2020deformable}} & ResNet50 &  39.3 & 19.8& 43.5&56.1\\
        \makecell[c]{DDetr w/o\\ multi-scale~\cite{zhu2020deformable}} & \modellight & 43.0 & 23.3& 46.3&61.2\\
        \bottomrule
    \end{tabular}
    \vspace{2pt}
    \caption{Comparison with DETR model over training epochs, mAP, inference time and GFLOPs.}
    \label{tab:detr_full}
\end{table}

% \begin{table} \small
% \setlength\tabcolsep{2pt}
%     \centering
%     \begin{tabular}{c|cccccccc}
%         \toprule
%         Method & \#Params(M)&FLOPs(G)& mAP & AP$_S$ & AP$_M$ & AP$_L$\\
%         \midrule
%         ResNet50 ~\cite{he2016deep} & 37.7 &239.232 & 36.5 &20.4& 40.3&48.1 &\\
%         ResNet101 ~\cite{he2016deep}& 56.7&319.07  & 38.5 &21.7& 42.8&50.4 &\\
%         X-101-32 ~\cite{xie2017aggregated}& 56.4&319.07 & 39.9 & 22.3 & 44.2 & 52.5 \\
%         X-101-64 ~\cite{xie2017aggregated}& 95.5&483.59 & 41.0 & 23.9 & 45.2 & 54.0 \\
%         \midrule
%         PVT-S ~\cite{wang2021pyramid} & 34.2& 226.5& 40.4 & 25.0 & 42.9 & 55.7 \\
%         ViL-S ~\cite{wang2021pyramid} & 35.6&252.2& 41.6 & 24.9 & 44.6 & 56.2 \\
%         SWIN-T ~\cite{wang2021pyramid} & 38.46 &244.82 & 41.5 & 26.4 & 45.1 & 55.7 \\
%         ViL-M ~\cite{wang2021pyramid} & 50.7&338.9& 42.9 & 27.0 & 46.1 & 57.2 \\
%         ViL-B ~\cite{wang2021pyramid} & 66.74&443.0& 44.3 & 28.9 & 47.9 & 58.3 \\
%         \midrule
%         \modellight& 6103&&43.8&27.4 &47.5 &58.5 \\
%         \bottomrule
%     \end{tabular}
%     \vspace{2pt}
%     \caption{We compare with large model variants of ResNet, pure transformer model and ResNet 50 by serving as a backbone for RetinaNet on COCO val 2017. Performance of RetinaNet~\cite{lin2017focal} on COCO~\cite{lin2014microsoft} val 2017. Comparison with ResNet~\cite{he2016deep} and RexNeXt~\cite{xie2017aggregated} model pretrained over ImageNet 1K.}
%     \label{tab:retinanet}
% \end{table}

\subsection{Self-supervised Learning DINO}
DINO is a recently proposed self-supervised learning framework. We adopt the default training setup in DINO to test the performance of \modellight on self-supervised learning.
We compare with ViT-S/16 model using DINO. Baseline model and \modellight are trained using 100 epoches with cosine schedule for learning rate and weight decay. Learning rate at the end of warmup is 0.0005 while weight decay at the end will be kept constant to 0.4. Batch size per GPU is set to 64. We report kNN accuracy as a metric to evaluate the performance of self-supervised model.

\section{1 line code change for Container-PAM}

\lstinputlisting[
    style       =   Python,
    caption     =   {With just 1 line of code change in the forward pass of the Attention module within ViT, one can implement \modelpam and obtain a +0.5 improvement on ImageNet top-1 accuracy.},
    label       =   {get_flops.tex}
]{get_flops.tex}

The attention code is borrowed from the TIMM library~\footnote{\texttt{https://github.com/rwightman/pytorch-image-models/tree/master/timm}}. The one-line code addition in the forward pass for \modelpam is implemented (and commented) in red. This code also requires enabling an additional parameter (also shown in red).

% \section{Code}
% We provide the implementation and training logs of the following main results:
% \begin{itemize}
%     \item IMAGENET pretraining to replicate 82.0 Top-1 accuracy of \modellight.
%     \item \modellight on RetinaNet and Mask RCNN
%     \item \modellight on SMCA-DETR
% \end{itemize}
